# Supplementary material for: Emergent flat band lattices in spatially periodic magnetic fields
Source: arXiv:1808.10046 ancillary file (2019-06-11)
Supplement: Supplementary file 1 [file supp.pdf]

# Supplemental Material for "Emergent flat band lattices in spatially periodic magnetic fields"

M. Tahir,[1] Olivier Pinaud,[2] and Hua Chen[1,3]

[1]*Department of Physics, Colorado State University, Fort Collins, CO 80523, USA*

[2]*Department of Mathematics, Colorado State University, Fort Collins, CO 80523, USA*

[3]*School of Advanced Materials Discovery,*
*Colorado State University, Fort Collins, CO 80523, USA*

## I. PLANE WAVE EXPANSION AND 2ND ORDER PERTURBATION FOR DIRAC ELECTRONS

We adopt a $\mathbf{k}\cdot\mathbf{p}$ description of 2D Dirac electrons in, e.g. graphene, subject to a general spatially periodic potential written in the basis of Pauli matrices

$$H = -i\hbar v_F(\tau_z\sigma_x\partial_x + \sigma_y\partial_y) + \mathbf{V}(\mathbf{r})\cdot\boldsymbol{\sigma} + V_0(\mathbf{r})\sigma_0, \tag{1}$$

where $\tau_z$ is the valley index. The potentials $\mathbf{V}$ and $V_0$ satisfy

$$\mathbf{V}(\mathbf{r}+\mathbf{R}) = \mathbf{V}(\mathbf{r}),\;\; V_0(\mathbf{r}+\mathbf{R}) = V_0(\mathbf{r}), \tag{2}$$

where $\mathbf{R} = n_1\mathbf{a}_1 + n_2\mathbf{a}_2$ is an arbitrary vector on the Bravais lattice $\{\mathbf{R}\}$ defined by the lattice vectors $\mathbf{a}_1$ and $\mathbf{a}_2$, $n_{1,2}\in\mathbb{Z}$.

Any wave functions can be expanded into plane waves

$$\psi_{\mathbf{r}} = \sum_{\mathbf{k}} c_{\mathbf{k}} e^{i\mathbf{k}\cdot\mathbf{r}}, \tag{3}$$

where $\mathbf{k}$ is an arbitrary complex vector, and both $\psi$ and $c$ are understood as $2\times 1$ column vectors. In contrast, because of the fixed periodicity of $\mathbf{V}$ and $V_0$, they can only be expanded into discrete Fourier components

$$\begin{aligned}\mathbf{V}(\mathbf{r}) &= \sum_{\mathbf{K}} \mathbf{V}_{\mathbf{K}} e^{i\mathbf{K}\cdot\mathbf{r}},\\ V_0(\mathbf{r}) &= \sum_{\mathbf{K}} V_{0\mathbf{K}} e^{i\mathbf{K}\cdot\mathbf{r}},\end{aligned} \tag{4}$$

where $\mathbf{K} = n_1\mathbf{b}_1 + n_2\mathbf{b}_2$ represents a vector in $\{\mathbf{K}\}$, the reciprocal lattice of $\{\mathbf{R}\}$, with

$$\mathbf{b}_1 = 2\pi\frac{\mathbf{a}_2\times\hat{z}}{(\mathbf{a}_1\times\mathbf{a}_2)\cdot\hat{z}},\;\; \mathbf{b}_2 = 2\pi\frac{\hat{z}\times\mathbf{a}_1}{(\mathbf{a}_1\times\mathbf{a}_2)\cdot\hat{z}}. \tag{5}$$

The inverse Fourier transform of $\mathbf{V}$ and $V_0$ gives

$$\begin{aligned}\mathbf{V}_{\mathbf{K}} &= \frac{1}{S}\int_{\text{cell}} d^2\mathbf{r} e^{-i\mathbf{K}\cdot\mathbf{r}}\mathbf{V}(\mathbf{r}),\\ V_{0\mathbf{K}} &= \frac{1}{S}\int_{\text{cell}} d^2\mathbf{r} e^{-i\mathbf{K}\cdot\mathbf{r}}V_0(\mathbf{r}),\end{aligned} \tag{6}$$

where $S$ is the total area of the unit cell. For the simplest case of one-dimensional single sinusoidal periodic potential proportional to $\sin(Kx)$, above equation gives $\mathbf{V}_{K\hat{x}} = -\mathbf{V}_{-K\hat{x}} \propto 1/2i$.

Substituting Eqs. (3), (4) and the Hamiltonian Eq. (1) into the eigen equation $H\psi = \epsilon\psi$, we have

$$
\begin{aligned}
0 &= \sum_{\mathbf{k}} \left[ \hbar v_F(\tau_z\sigma_x k_x + \sigma_y k_y)c_{\mathbf{k}} + \sum_{\mathbf{K}'}(\mathbf{V}_{\mathbf{K}'}\cdot\boldsymbol{\sigma} + V_{0\mathbf{K}'}\sigma_0)c_{\mathbf{k}-\mathbf{K}'} - \epsilon c_{\mathbf{k}} \right] e^{i\mathbf{k}\cdot\mathbf{r}} \qquad (7)\\
&\equiv \sum_{\mathbf{k}} \left[ H_0(\mathbf{k})c_{\mathbf{k}} + \sum_{\mathbf{K}'} V(\mathbf{K}')c_{\mathbf{k}-\mathbf{K}'} - \epsilon c_{\mathbf{k}} \right] e^{i\mathbf{k}\cdot\mathbf{r}}
\end{aligned}
$$

or equivalently

$$
H_0(\mathbf{k})c_{\mathbf{k}} + \sum_{\mathbf{K}'} V(\mathbf{K}')c_{\mathbf{k}-\mathbf{K}'} - \epsilon c_{\mathbf{k}} = 0, \qquad (8)
$$

which must be solved for each $\mathbf{k}$. We can restrict $\mathbf{k}$ to be within the "superlattice" Brillouin zone defined by $\mathbf{b}_1$ and $\mathbf{b}_2$ by replacing $\mathbf{k}$ with $\mathbf{k}+\mathbf{K}$, where $\mathbf{K}$ can take any value in $\{\mathbf{K}\}$:

$$
[H_0(\mathbf{k}+\mathbf{K}) + V(0)]\, c_{\mathbf{k}+\mathbf{K}} + \sum_{\mathbf{K}'\neq 0} V(\mathbf{K}')c_{\mathbf{k}+\mathbf{K}-\mathbf{K}'} - \epsilon c_{\mathbf{k}+\mathbf{K}} = 0. \qquad (9)
$$

Note that although there may only be finite number of terms in the summation over $\mathbf{K}'$, e.g. $V(\mathbf{r})$ has only two Fourier components, $\mathbf{K}$ can take infinite number of values as long as $\mathbf{K} \in \{\mathbf{K}\}$. Therefore Eq. (9) corresponds to an infinite-dimension matrix equation. Each $2\times 2$ diagonal block is $H_0(\mathbf{k}+\mathbf{K}) + V(0) - \epsilon$, which is coupled to other diagonal blocks of $H_0(\mathbf{k}+\mathbf{K}-\mathbf{K}') + V(0) - \epsilon$ through $V(\pm\mathbf{K}')$. $V_{\mathbf{K}'} = V^{\dagger}_{-\mathbf{K}'}$ because $V(\mathbf{r})$ is Hermitian. In reality, however, $\mathbf{K}$ is limited by the portion near the original Brillouin zone corners in which the band dispersion is approximately linear. Written into a matrix form $[H(\mathbf{k}) - \epsilon]c_{\mathbf{k}} = 0$, the matrix Hamiltonian $H(\mathbf{k})$ looks like

$$
H(\mathbf{k}) = \begin{pmatrix}
H_0(\mathbf{k}) + V(0) & \dots & V(\mathbf{K}') & & & \\
\vdots & \ddots & & & & \\
V(-\mathbf{K}') & & H_0(\mathbf{k}-\mathbf{K}') + V(0) & \dots & V(\mathbf{K}'') & \\
& & \vdots & \ddots & & \\
& & V(-\mathbf{K}'') & & H_0(\mathbf{k}-\mathbf{K}'-\mathbf{K}'') + V(0) & \\
& & & & & \ddots
\end{pmatrix} \qquad (10)
$$

If we are interested in the influence on $H_0(\mathbf{k})$ due to a weak periodic potential, a good approximation can be achieved by considering only the nearest neighboring images $H_0(\mathbf{k}-\mathbf{K}')$ where $\mathbf{K}'$ corresponds to the nonzero Fourier components $V_{\mathbf{K}'}$. To check consistency one will have to systematically take into account the indirect couplings to $H_0(\mathbf{k}+\mathbf{K}-\mathbf{K}')$ and check

convergence. In this first-shell approximation, Eq. (9) becomes a finite-dimension matrix equation with the dimension $2(n_{\mathbf{K}'}+1)$, where $n_{\mathbf{K}'}$ is the number of Fourier components in $V(\mathbf{r})$. The matrix Hamiltonian looks like

$$H(\mathbf{k})=\begin{pmatrix} H_0(\mathbf{k})+V(0) & V(\mathbf{K}') & \dots & V(\mathbf{K}'') \\ V(-\mathbf{K}') & H_0(\mathbf{k}-\mathbf{K}')+V(0) & & \\ \vdots & & \ddots & \\ V(-\mathbf{K}'') & & & H_0(\mathbf{k}-\mathbf{K}'')+V(0) \end{pmatrix} \tag{11}$$

If $V(\mathbf{K}')$ is small and $k\to 0$, one can further use 2nd order perturbation to arrive at an effective $2\times 2$ Hamiltonian based on Eq. (11):

$$H_{\text{eff}}(\mathbf{k})=H_0(\mathbf{k})+V(0)-\sum_{\mathbf{K}'}V(\mathbf{K}')\left[H_0(\mathbf{k}-\mathbf{K}')+V(0)\right]^{-1}V^\dagger(\mathbf{K}'). \tag{12}$$

For the Dirac Hamiltonian and the cosinusoidal magnetic field used in the main text, with $\hbar v_F K$ and $K$ the units of energy and of wave vector, respectively, Eq. (12) becomes

$$H^D_{\text{eff}}(\mathbf{k})=H^D_0(\mathbf{k})-\sum_{\mathbf{K}'}V(\mathbf{K}')[H^D_0(\mathbf{k}-\mathbf{K}')]^{-1}V^\dagger(\mathbf{K}'), \tag{13}$$

where $H^D_0(\mathbf{k})=\mathbf{k}\cdot\boldsymbol{\sigma}$, $\mathbf{K}'=\pm\hat{x}$, $\pm\hat{y}$, and

$$V(\pm\hat{x})=\pm\frac{\phi}{2i}\sigma_y,\ V(\pm\hat{y})=\mp\frac{\phi}{2i}\sigma_x \tag{14}$$

with $\phi\equiv eB/\hbar K^2$. Expanding Eq. (13) up to the 1st order in $k$, we obtain

$$H^D_{\text{eff}}(\mathbf{k})=H^D_0(\mathbf{k})(1-\phi^2)+O\left(k^2\right). \tag{15}$$

As discussed in the main text this result is valid when $\phi\ll 1$.

## II. ANALYTIC RESULT FOR THE NEAR-ZERO-ENERGY STATES OF DIRAC ELECTRONS IN A 2D PERIODIC MAGNETIC FIELD

We follow the approach introduced in [1, 2]. Consider a 2D Dirac system in the presence of a 2D spatially periodic magnetic field $B$ that varies smoothly on a scale much larger than the lattice constant. The Dirac Hamiltonian in the long-wave length limit is

$$H=v_F\boldsymbol{\sigma}\cdot[-i\hbar\nabla+e\mathbf{A}(\mathbf{r})] \tag{16}$$

The periodicity of $\mathbf{A}(\mathbf{r})$ defines a new Bravais lattice as discussed in the previous section.

The Fourier components of the $z$ component of the periodic magnetic field are

$$B_{\mathbf{K}'} = \frac{1}{S}\int_{\text{cell}} d^2\mathbf{r} e^{-i\mathbf{K}'\cdot\mathbf{r}} B(\mathbf{r}). \tag{17}$$

Note that $B_{\mathbf{K}'=\mathbf{0}} = 0$ due to the zero spatial average, and that $B_{\mathbf{K}'} = -B^*_{\mathbf{K}'}$ because $\mathbf{B}(\mathbf{r})$ is real.

The zero-energy eigenstates of the Hamiltonian in Eq. (16) can be written as $\Psi = (\phi_+, \phi_-)$ which solve the following differential equation

$$\left[\partial_x \pm i\partial_y + i(\lambda_x \pm i\lambda_y)\right]\phi_\pm = 0 \tag{18}$$

where $\lambda = e\mathbf{A}/\hbar$. Using the Coulomb gauge, Eq. (18) subject to periodic boundary condition is solved by

$$\phi_\pm(\mathbf{r}) = g_\pm \exp[\pm\chi(\mathbf{r})] \tag{19}$$

where $g_\pm$ are constants. $\chi(\mathbf{r})$ is

$$\chi(\mathbf{r}) = -\frac{e}{\hbar}\sum_{\mathbf{K}'\neq\mathbf{0}} \frac{B_{\mathbf{K}'}}{|\mathbf{K}'|^2} e^{i\mathbf{K}'\cdot\mathbf{r}}. \tag{20}$$

For our magnetic field there exists two solutions [1]

$$\Psi_{+,0} = C_+\begin{pmatrix} e^{\chi(\mathbf{r})} \\ 0 \end{pmatrix}, \Psi_{-,0} = C_-\begin{pmatrix} 0 \\ e^{-\chi(\mathbf{r})} \end{pmatrix}, \tag{21}$$

where the normalization constants are

$$C_\pm = \left[\int_{\text{cell}} d^2\mathbf{r} e^{\pm 2\chi(\mathbf{r})}\right]^{-\frac{1}{2}}. \tag{22}$$

Above results are solved for $\mathbf{k} = 0$. To get the dispersion one simply takes $\mathbf{k}\cdot\boldsymbol{\sigma}$ as a perturbation in this zero energy subspace. The effective Hamiltonian is obtained as

$$H^{\text{eff}} = \frac{v_F^{\text{eff}}}{v_F}\boldsymbol{\sigma}\cdot\mathbf{k}, \qquad v_F^{\text{eff}} = v_F S C_+ C_-. \tag{23}$$

For the vector potential used in the main text one can get an analytic form of $C_\pm$, and finally obtain

$$v_F^{\text{eff}} = \frac{v_F}{[I_0(2\phi)]^2}. \tag{24}$$

The asymptotic form of Eq. (24) at large $\phi$ can be obtained using the approximation

$$I_0(x) \approx \frac{e^x}{\sqrt{2\pi x}}\left(1 + \frac{1}{8x}\right). \tag{25}$$

## III. SQUARE SUPERLATTICE FOR SCHRÖDINGER ELECTRONS FORMED BY PERIODIC MAGNETIC FIELDS

The Schrödinger Hamiltonian in the presence of a periodic magnetic field is

$$\begin{aligned} H &= \frac{\hbar^2}{2m}\left(-i\nabla + \frac{e}{\hbar}\mathbf{A}\right)^2 + \frac{g\mu_B}{2}\boldsymbol{\sigma}\cdot\mathbf{B}(\mathbf{r}) \\ &= H_0 + V, \end{aligned} \tag{26}$$

where the 2nd term is the Zeeman coupling between spin and the magnetic field. If one ignores spin-orbit coupling, for a single spin species the Zeeman term simply behaves as a scalar potential. Assuming the magnetic field is along $\hat{z}$, the field-induced perturbation is

$$V = -\frac{ie\hbar}{m}\mathbf{A}\cdot\nabla + \frac{e^2}{2m}|\mathbf{A}|^2 + \frac{g\mu_B}{2}B(\mathbf{r}), \tag{27}$$

The Fourier transform of $V$ is

$$\begin{aligned} V_{\mathbf{K}'} &= \frac{1}{S}\int_{\text{cell}} d^2\mathbf{r}e^{-i\mathbf{K}'\cdot\mathbf{r}}V \\ &= \frac{1}{S}\int_{\text{cell}} d^2\mathbf{r}\left[\frac{e\hbar}{m}\mathbf{A}\cdot(\mathbf{k}+\mathbf{K}-\mathbf{K}') + \frac{e^2}{2m}|\mathbf{A}|^2 + \frac{g\mu_B}{2}B\right]e^{-i\mathbf{K}'\cdot\mathbf{r}}, \end{aligned} \tag{28}$$

where the $\mathbf{k}+\mathbf{K}-\mathbf{K}'$ in the first term is because the gradient operator is actually acting on the plane wave $e^{i(\mathbf{k}+\mathbf{K}-\mathbf{K}')\cdot\mathbf{r}}$ since the secular equation in the plane wave basis is

$$\sum_{\mathbf{k},\mathbf{K}}\left[H_0(\mathbf{k}+\mathbf{K})c_{\mathbf{k}+\mathbf{K}} + \sum_{\mathbf{K}'}V(\mathbf{K}')c_{\mathbf{k}+\mathbf{K}-\mathbf{K}'} - \epsilon c_{\mathbf{k}+\mathbf{K}}\right]e^{i(\mathbf{k}+\mathbf{K})\cdot\mathbf{r}} = 0. \tag{29}$$

Because of the $|\mathbf{A}|^2$ in the 2nd term in the integrand, there are more Fourier components than that included in $\mathbf{A}$. For the square lattice magnetic field used in the main text, we have ($\mathbf{K}' = n\hat{x}, n\hat{y}$, with $n = 0, \pm 1, \pm 2$)

$$\begin{aligned} V(0) &= \frac{e^2B^2}{2mK^2} = \frac{m\omega_c^2}{2K^2}, \\ V(\pm\hat{x}) &= \pm\frac{\hbar\omega_c}{2i}\frac{(k_y+K_y)}{K} + \frac{g\mu_B}{4}B, \\ V(\pm\hat{y}) &= \mp\frac{\hbar\omega_c}{2i}\frac{(k_x+K_x)}{K} + \frac{g\mu_B}{4}B, \\ V(\pm 2\hat{x}) &= V(\pm 2\hat{y}) = -\frac{e^2B^2}{8mK^2} = -\frac{m\omega_c^2}{8K^2}. \end{aligned} \tag{30}$$

Here $\omega_c = eB/m$, $m$ is the effective mass of electrons, $\mu_B = e\hbar/2m_e$, $m_e$ the mass of electron in vacuum, $g$ an effective $g$-factor, and $H_0(\mathbf{k}) = \hbar^2k^2/2m$. If we use $\hbar^2K^2/2m$ as the units

of energy, and $K$ as the units of wave vector, all terms in the secular equation become dimensionless, with

$$\begin{aligned}
&H_0(\mathbf{k}+\mathbf{K}) = (\mathbf{k}+\mathbf{K})^2, \\
&V(0) = \phi^2, \\
&V(\pm\hat{x}) = \mp i\phi(k_y + K_y) + \frac{g}{4}\frac{m}{m_e}\phi, \\
&V(\pm\hat{y}) = \pm i\phi(k_x + K_x) + \frac{g}{4}\frac{m}{m_e}\phi, \\
&V(\pm 2\hat{x}) = V(\pm 2\hat{y}) = -\frac{\phi^2}{4}.
\end{aligned} \tag{31}$$

When $g = 0$ in Eq. (31), we obtain the Eq. (11) in the main text.
2nd order perturbation using above expressions with $g = 0$ gives

$$H_{\text{eff}}(\mathbf{k}) = k^2\left(1 - 2\phi^2\right) + \phi^2 + O\left(k^4\right). \tag{32}$$

The 2nd term is due to the fact that $|\mathbf{A}(\mathbf{r})|^2$ has a nonzero spatial average. Thus the approximate magic value for Schrödinger electrons is

$$\phi = \frac{1}{\sqrt{2}}, \tag{33}$$

which will give a flat band located at finite energy $\phi^2$, as shown in Fig. 2 of the main text.

## IV. TRIANGULAR SUPERLATTICE FOR DIRAC AND SCHRÖDINGER ELECTRONS FORMED BY PERIODIC MAGNETIC FIELDS

A triangular superlattice can be formed by the following (cosinusoidal) perpendicular magnetic field:

$$\mathbf{B} = B\hat{z}\sum_{i=1}^{3}\cos(\mathbf{K}_i\cdot\mathbf{r}) \tag{34}$$

with

$$\mathbf{K}_1 = K\hat{x},\ \mathbf{K}_2 = K\left(\frac{1}{2}\hat{x} + \frac{\sqrt{3}}{2}\hat{y}\right),\ \mathbf{K}_3 = K\left(-\frac{1}{2}\hat{x} + \frac{\sqrt{3}}{2}\hat{y}\right) \tag{35}$$

The corresponding vector potential $\mathbf{A}$ in the Coulomb gauge is

$$\mathbf{A}(\mathbf{r}) = \frac{B}{K^2}\sum_{i=1}^{3}\sin(\mathbf{K}_i\cdot\mathbf{r})\hat{z}\times\mathbf{K}_i \tag{36}$$

In the notation introduced in Sec. I, we have periodic potential for Dirac electrons

$$\mathbf{V}(\mathbf{r}) = ev_F\mathbf{A}(\mathbf{r}), \tag{37}$$

which has six Fourier components in the dimensionless form:

$$\begin{aligned}\mathbf{V}(\pm\mathbf{K}_1) &= \pm\frac{\phi}{2i}\hat{y}, \\ \mathbf{V}(\pm\mathbf{K}_2) &= \pm\frac{\phi}{2i}\left(-\frac{\sqrt{3}}{2}\hat{x}+\frac{1}{2}\hat{y}\right), \\ \mathbf{V}(\pm\mathbf{K}_3) &= \pm\frac{\phi}{2i}\left(-\frac{\sqrt{3}}{2}\hat{x}-\frac{1}{2}\hat{y}\right).\end{aligned} \tag{38}$$

Using 2nd-order perturbation theory with the 1st shell approximation we arrive at the effective Hamiltonian

$$H^D_{\text{eff}}(\mathbf{k}) = H^D_0(\mathbf{k})\left(1-\frac{3\phi^2}{2}\right)+O(k^2), \tag{39}$$

which is valid at small $\phi$. Numerical results for larger $\phi$ using the plane wave approach are shown in Fig. 1.

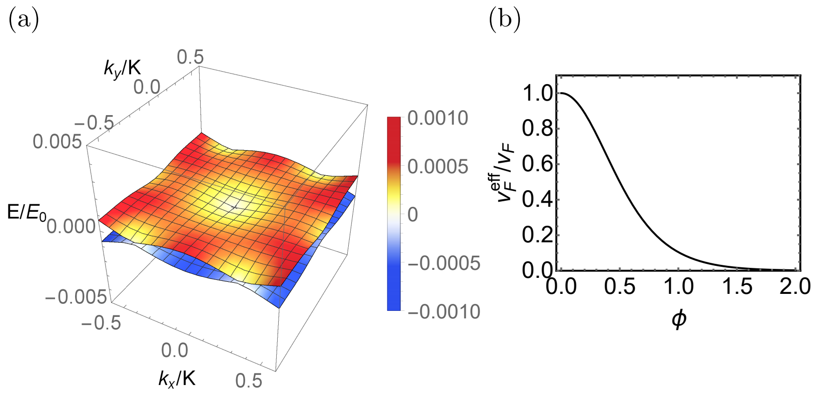


FIG. 1. Flat bands for Dirac electrons in triangular periodic magnetic fields. (a) Band structure for the two particle-hole symmetric bands close to zero energy when $\phi = 2$. $E_0 = \hbar v_F K$ is the energy unit. The color scale is the same as $E/E_0$. (b) Renormalized Fermi velocity $v_F^{\text{eff}}$ vs. $\phi$. A plane wave cutoff of $K_c = 5K$ is used.

Similarly, a triangular superlattice can be formed by periodic magnetic fields for Schrödinger

electrons. Following the formulation used in previous section, the Fourier components are

$$\begin{aligned}
&V(0) = \frac{3}{2}\phi^2, \\
&V(\pm\mathbf{K}_1) = \mp i\phi(\mathbf{k}+\mathbf{K})\cdot\hat{y} + \frac{g}{4}\frac{m}{m_e}\phi, \\
&V(\pm\mathbf{K}_2) = \mp i\phi(\mathbf{k}+\mathbf{K})\cdot\left(-\frac{\sqrt{3}}{2}\hat{x} + \frac{1}{2}\hat{y}\right) + \frac{g}{4}\frac{m}{m_e}\phi, \\
&V(\pm\mathbf{K}_3) = \mp i\phi(\mathbf{k}+\mathbf{K})\cdot\left(-\frac{\sqrt{3}}{2}\hat{x} - \frac{1}{2}\hat{y}\right) + \frac{g}{4}\frac{m}{m_e}\phi, \\
&V(\pm 2\mathbf{K}_1) = V(\pm 2\mathbf{K}_2) = V(\pm 2\mathbf{K}_3) = -\frac{\phi^2}{4}, \\
&V(\mathbf{K}_1 \pm \mathbf{K}_2) = -V(\mathbf{K}_1 \pm \mathbf{K}_3) = V(\mathbf{K}_2 \pm \mathbf{K}_3) = \mp\frac{\phi^2}{4}.
\end{aligned} \tag{40}$$

For the triangular lattice of Schrödinger electrons, numerical results using the plane wave approach are shown in Fig. 2.

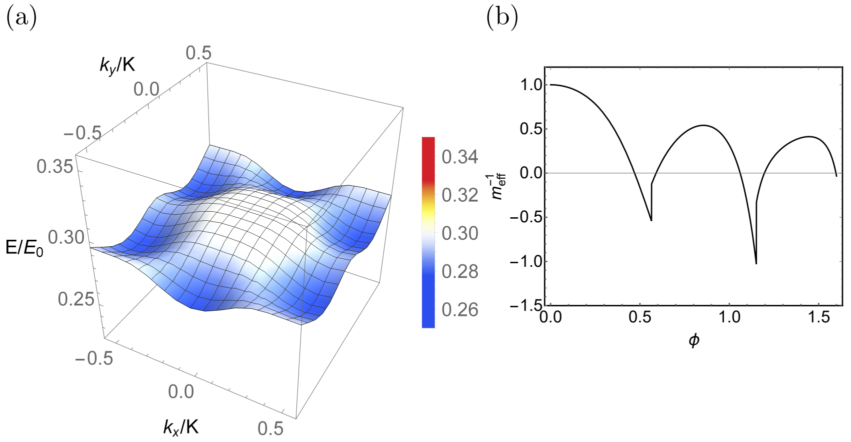


FIG. 2. Flat bands for 2DEG in triangular periodic magnetic fields. (a) Band structure for the lowest band when $\phi = 0.47$ near the first magic value. $E_0 = \hbar^2 K^2/2m$ is the energy unit. The color scale is the same as $E/E_0$ with white corresponding to the energy at $\mathbf{k} = 0$. (b) Renormalized inverse effective mass $m_{\rm eff}^{-1}$ (in units of $m^{-1}$) vs. $\phi$. A plane wave cutoff of $K_c = 7K$ is used.

## V. TIGHT-BINDING MODEL FOR SCHRÖDINGER ELECTRONS UNDER PERIODIC MAGNETIC FIELDS

Figure 3 shows the band structure and density of states of the square lattice tight-binding model for Schrödinger electrons, Eq. (24) in main text. Since the flat bands occur near

$\phi = \pi/8$, we define a dimensionless parameter $\alpha \equiv 1 - 8\phi/\pi$ and consider small values of $\alpha$. The band structure is plotted for $\alpha = 0.01$, while in the DOS plot we included $\alpha$ =0.03, 0.02, and 0.05.

Near $\alpha = 0$ we can redefine $(k_x + k_y)/2 = k_\parallel, (k_x - k_y)/2 = k_\perp$, and expand $\epsilon_\pm(\mathbf{k}) = 4t \pm |h_\mathbf{k}|$ for small $k_\perp$. The result is

$$\epsilon_\pm(\mathbf{k}) \approx 4t \pm 2\sqrt{2}t \left[ \sqrt{1+\cos(8\phi)} |\cos(k_\parallel a)| - \frac{\cos(8\phi) + \cos(2k_\parallel a)}{2\sqrt{1+\cos(8\phi)}|\cos(k_\parallel a)|} k_\perp^2 a^2 \right] + O(k_\perp^3). \tag{41}$$

Thus there is no linear in $k_\perp$ term as long as $\phi \neq \pi/8$ and $k_\parallel \neq \pi/2a$, and the density of states will be large at the band edge. However, when $\phi = \pi/8$, $\epsilon_\pm(\mathbf{k}) \approx 4t \pm 4at|\sin(k_\parallel a) k_\perp| + O(k_\perp^3)$, while $\epsilon_\pm(\mathbf{k}) \approx 4t \pm 4at|\sin(\phi) k_\perp| + O(k_\perp^3)$ when $k_\parallel = \pi/2a$. The former corresponds to Dirac line nodes along $k_\parallel$, while the latter corresponds to asymmetric Dirac cone at $k_\parallel = \pm\pi/2a$.

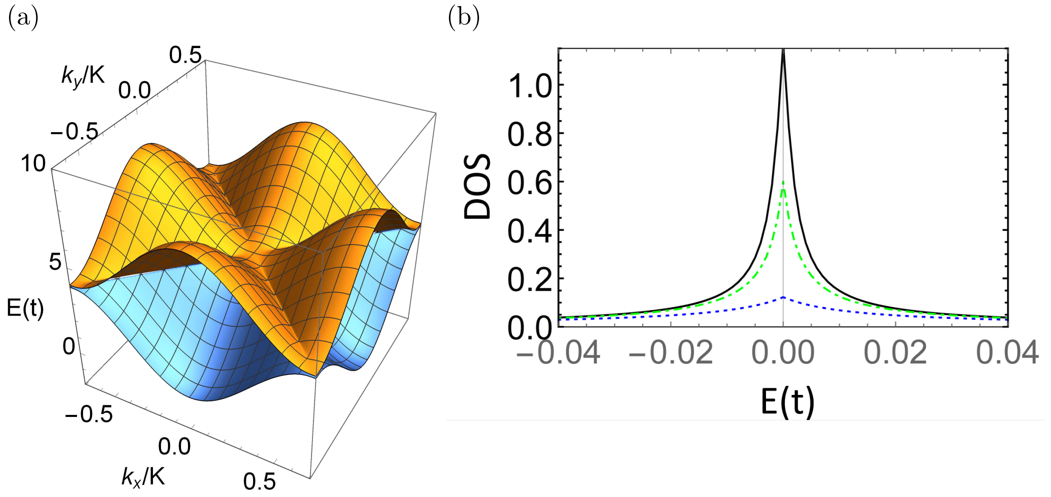


FIG. 3. Low-energy band structure (a) and DOS (b) of the square lattice tight-binding model with staggered fluxes. The band structure is for $\alpha = 0.01$, while in the DOS plot the solid, dot-dashed, and dotted curves respectively correspond to $\alpha = 0.003$, 0.02, and 0.05. A Gaussian broadening of $0.002t$ is used for (b).

## VI. DESCRIPTION OF THE TIGHT-BINDING HAMILTONIAN FILES

The tight-binding Hamiltonian for the Schrödinger electron case with $\phi = 0.6$ written in the Wannier function basis (Fig. 4 in the main text) is stored in the text file

"`hmat-2band.dat`". Every four rows in the file describe the Hamiltonian block of $\langle\phi_i(\mathbf{0})|H|\phi_j(\mathbf{R})\rangle$, where $i, j = 1, 2$ label the two Wannier functions, and $\mathbf{R}$ is a Bravais lattice vector. The first two numbers in the 2nd row of each block are the coordinates of $\mathbf{R}$ in units of $1/K$, while the third number is $|\mathbf{R}|$ according to which the blocks are sorted. The 3rd and 4th rows in each block are the complex matrix elements $\langle\phi_i(\mathbf{0})|H|\phi_j(\mathbf{R})\rangle$ in units of $\hbar^2K^2/2m$. For example, the 2nd column of the 3rd row in each block is $\langle\phi_1(\mathbf{0})|H|\phi_2(\mathbf{R})\rangle$.

"`hmat-3band.dat`" is the tight-binding Hamiltonian for the lowest three bands of the Schrödinger electron case with Zeeman coupling ($gm/m_e = 1.0$) and $\phi = 0.67$ written in the Wannier function basis shown in Fig. 8 of the main text. The structure of the file is the same as the 2-band case except that each block is 5 rows because of the larger basis.

## VII. MAXIMALLY-LOCALIZED WANNIER FUNCTIONS FOR THE TWO LOWEST BANDS OF THE SCHRÖDINGER CASE

The maximally localized Wannier functions for the two lowest bands in the Schrödinger case are shown in Fig. 4. Although the initial guess of the two Wannier functions was chosen as two Gaussian functions located at $(\pi/K, 0)$ and $(0, \pi/K)$, after running the localization routine they evolve to the form more compatible with the four-fold rotational symmetry with respect to the origin.


[1] R. Jackiw, Phys. Rev. D **29**, 2375 (1984).

[2] I. Snyman, Phys. Rev. B **80**, 054303 (2009).

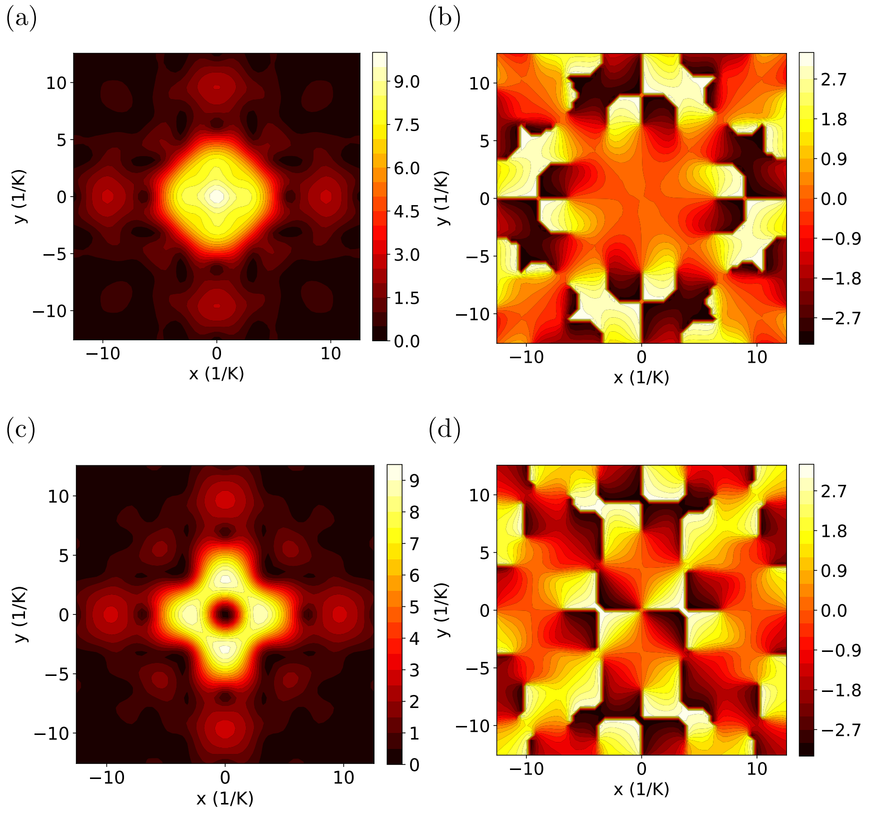


FIG. 4. Norm (a and c) and phase (b and d) of the MLWFs of the lowest 2 bands of a 2DEG. $\phi = 0.6$. A plane wave cutoff of $K_c = 9K$ and a Brillouin zone discretization of $11 \times 11$ were used.
